# Supplementary material for: CurveCloudNet: Processing Point Clouds with 1D Structure
Source: arXiv:2303.12050 source file (2024-02-01)
Supplement: Supplementary file 1 [file shapenet-seg.tex]

\begin{table*}[t]
\setlength{\tabcolsep}{4pt}
\centering
\scalebox{0.93}{
    \begin{tabular}{ l | c | c c c | c c c}
    \toprule
    & \multicolumn{4}{c}{\textbf{Class-Averaged mIoU ($\uparrow$)}} & \multicolumn{3}{c}{\textbf{{ Performance}}} \\
    \textbf{Method} & Mean & Parallel & Grid & Random & Time \scriptsize (ms) ($\downarrow$) & GPU \scriptsize (GB) ($\downarrow$) & Param \scriptsize (M)) \\
    \midrule
    PointNet~\cite{Qi2017CVPR} & 80.1 & 80.8 \scriptsize $\pm$ 0.0 & 80.6 \scriptsize $\pm$ 0.5 & 78.9 \scriptsize $\pm$ 0.1 & 8 & 0.16 & 1.5 \\
    PointNet++~\cite{Qi2017NIPS} & 80.1 & 81.8 \scriptsize $\pm$ 0.1 & 80.1 \scriptsize $\pm$ 0.04 & 78.3 \scriptsize $\pm$ 0.7 & 59 & 0.91 & 1.5 \\
    DGCNN~\cite{Wang2019SIGGRAPHb} & 80.2 & 81.2 \scriptsize $\pm$ 0.2 & 80.9 \scriptsize $\pm$ 0.02 & 78.6 \scriptsize $\pm$ 0.3 & 80 & 0.79 & 21.8 \\
    CurveNet~\cite{Xiang2021ICCV} & 82.8 & \textbf{84.0} \scriptsize $\pm$ 0.2 & \textbf{83.8} \scriptsize $\pm$ 0.4 & 80.6 \scriptsize $\pm$ 0.2 & 237 & 1.27 & 5.5 \\
    PointMLP~\cite{Ma2022ICLR} & 80.9 & 82.2 \scriptsize $\pm$ 0.3 & 81.3 \scriptsize $\pm$ 0.3 & 79.3 \scriptsize $\pm$ 0.3 & 57 & 0.89 & 16.8 \\
    PointNext-S~\cite{Qian2022PointNeXtRP} & 82.8 & 83.8 \scriptsize $\pm$ 0.1 & 83.1 \scriptsize $\pm$ 0.3 & 81.5 \scriptsize $\pm$ 0.2 & 79 & 1.83 & 13.8 \\
    \hline  % we use PointNextS-C160 variant!
    % PVCNN~\cite{Liu2019NeurIPS} & \textbf{83.8} \scriptsize $\pm$ 0.3 & 83.2 \scriptsize $\pm$ 0.1 & 81.6 \scriptsize $\pm$ 0.0 & 32 & 1.02 & 4.2 \\
    MinkowskiNet~\cite{Choy2019CVPR} & 81.1 & 82.6  \scriptsize $\pm$ 0.3 & 82.0  \scriptsize $\pm$ 0.5 & 80.1  \scriptsize $\pm$ 0.5 & 40 & 0.19 & 36.6 \\
    Cylinder3D~\cite{Zhou2020ARXIV} & 79.6 & 81.2 \scriptsize $\pm$ 0.1 & 80.1 \scriptsize $\pm$ 0.0 & 77.6 \scriptsize $\pm$ 0.1 & 96 & 6.20 & 56.0 \\ 
    Cylinder3D (ours) & 81.4 & 82.8 \scriptsize $\pm$ 0.0 & 81.6 \scriptsize $\pm$ 0.0 & 80.1 \scriptsize $\pm$ 0.1 & 80 & 6.20 & 56.0 \\ 
    SphereFormer~\cite{lai2023spherical} & 79.5 & 80.3 \scriptsize $\pm$ 0.3 & 79.9 \scriptsize $\pm$ 0.4 & 78.3 \scriptsize $\pm$ 0.4 & 38 & 0.19 & 32.3 \\
    \hline
    CurveCloudNet & \textbf{83.1} & 83.7 \scriptsize $\pm$ 0.2 & 83.6 \scriptsize $\pm$ 0.5 & \textbf{81.9} \scriptsize $\pm$ 0.3 & 68 & 1.03 & 11.7\\
    \bottomrule
    \end{tabular}}
    \vspace{1mm}
    \caption{\textit{Object Segmentation Results.} Class-average mIoU is reported for three curve sampling patterns (\textit{parallel} and \textit{grid} and \textit{random}) on all 16 object categories spanning 50 object parts of the ShapeNet Part Segmentation Dataset. CurveCloudNet outperforms all baselines in terms of mIoU for the \textit{grid} and the \textit{random} curve sampling pattern, while performing on par with the best-performing PVCNN~\cite{Liu2019NeurIPS} for the case of \textit{parallel} sampling. Performance is on an Nvidia RTX 3090 GPU (batch size 16).}
    \label{tab:shapenet-segmentation}
\end{table*}

% \begin{table*}[t]
% \setlength{\tabcolsep}{4pt}
% \centering
% \scalebox{0.93}{
%     \begin{tabular}{ l | c c | c c | c c | c c c}
%     \toprule
%     & \multicolumn{6}{c}{\textbf{IoU ($\uparrow$)}} & \multicolumn{3}{c}{\textbf{{ Performance}}} \\
%     & \multicolumn{2}{c}{Parallel} & \multicolumn{2}{c}{Grid} & \multicolumn{2}{c}{Random} & & & \\
%     \textbf{Method} & Class  & Instance & Class & Instance & Class & Instance & Time \scriptsize (ms) ($\downarrow$) & GPU \scriptsize (GB) ($\downarrow$) & Param \scriptsize (M)) \\
%     \midrule
%     % PointNet~\cite{Qi2017CVPR} & \textbf{96.3 \scriptsize $\pm$ 0.1} & 99.1 \scriptsize $\pm$ 0.08 & 95.4 \scriptsize $\pm$ 0.3 & 1 & 0.12 & 1.3 \\
%     % PointNet++~\cite{Qi2017NIPS} & 95.3 \scriptsize $\pm$ 0.7 & 99.0 \scriptsize $\pm$ 0.05 & 95.5 \scriptsize $\pm$ 0.6 & 51 & 0.91 & 1.6 \\
%     % DGCNN~\cite{Wang2019SIGGRAPHb} & 93.7 \scriptsize $\pm$ 0.5 & 98.9 \scriptsize $\pm$ 0.03 & 93.6 \scriptsize $\pm$ 0.5 & 73 & 0.78 & 0.6 \\
%     % PointMLP~\cite{Ma2022ICLR} & 94.8 \scriptsize $\pm$ 1.3 & 99.2 \scriptsize $\pm$ 0.05 & 95.3 \scriptsize $\pm$ 1.0 & 54 & 0.76 & 13.2 \\
%     PVCNN~\cite{Liu2019NeurIPS} ~ & 71.0 & 81.8 & 70.9 & 81.3 & 68.3 & 79.9 & & & \\ \hline
%     CurveCloudNet & 71.1 & 81.4 & 71.0 & 80.9 & 68.3 & 79.9 & 95 & 1.16 & 8.7\\
%     \bottomrule
%     \end{tabular}}
%     \vspace{1mm}
%     \caption{\textit{Object Segmentation Results.}}
%     \label{tab:shapenet-classification}
% \end{table*}
